# Supplementary material for: Meta-INR: Efficient Encoding of Volumetric Data via Meta-Learning Implicit Neural Representation
Source: arXiv:2502.09669 source file (2025-02-12)
Supplement: Supplementary file 1 [file appendix.tex]

\newpage
\clearpage
\section*{Appendix}

\setcounter{section}{0}
\setcounter{figure}{0}
\setcounter{table}{0}
\setcounter{page}{0}

\section{Additional results}
